# Supplementary material for: Do We Really Need Complicated Model Architectures For Temporal Networks?
Source: arXiv:2302.11636 source file (2023-02-22)
Supplement: Supplementary file 1 [file data_alignment.tex]

\section{data alignment}

\begin{definition} [Algorithmic alignment] \label{definition:algorithmic_alignment}
Let us suppose $F(x) = f_L(f_{L-1}(\ldots f_1(x_i)\ldots))$ is the target function which could be decomposed into $L$ sub-task functions, and $G(x)= g_L(g_{L-1}(\ldots g_1(x)\ldots))$ is the neural network with $L$ modules.
Let $\mathcal{S}(f, g, \epsilon, \delta)$ denotes the sample complexity of approximating $f$ with $g$ and achieve $\mathbb{E}_{x\sim \mathcal{D}} \| f(x) - g(x) \|_2\leq \epsilon$ with probability at least $1-\delta$.
Then, we say the neural network $G$ and target function $F$ are $(M, \epsilon, \delta)$-algorithmic aligned if $\max_{\ell\in[L]}~\mathcal{S}(f_\ell, g_\ell, \epsilon, \delta) \leq M/L$.
\end{definition}

The idea of algorithm alignment (Definition~\ref{definition:algorithmic_alignment}) is originally studied in~\cite{xu2019can}, in which they show that a better generalization could be achieved if the ``computation structure'' of the neural network model aligns with the ``algorithmic structure'' of the underlying function to reason about. 
More specifically, \cite{xu2019can} shows that if neural network $G$ is algorithmic aligned with the target function $F$ and each neural network module $g_\ell$ could learn its corresponding target sub-task function $f_\ell$ with at most $M/L$ samples and achieve error $\epsilon$ with probability at least $1-\delta$, then under some assumptions on the model's Lipschitzness and training strategy (Assumption~\ref{assumption:algorithmic_alignment_assmption}), we know the whole neural network model $G$ can learn the overall target function $F$ with at most $M$ samples and achieve error $\mathcal{O}(\epsilon)$ with probability at least $1-\mathcal{O}(\delta)$.
In this paper, we study a special case (namely data alignment) which captures the alignment between the data inputs and their labels.
More specifically, we shown in Proposition~\ref{prop:data_alignment}, if we could encode appropriate non-linearities of the first $m$ sub-task target function into model's input features via domain expertise, then the new neural network model $G^\prime$ only requires at most $M(L-m)/L$ samples to learn the overall target function $F$.

\begin{proposition} (Data alignment improves sample complexity) \label{prop:data_alignment}
Suppose neural network $G(x)$ and  target function $F(x)$ are $(M, \epsilon, \delta)$-algorithmic aligned.
If we can encode part of the sub-task target function $z = f_m(f_{m-1}(\ldots f_1(x)\ldots))$ into the input data for any $m\leq L$ by replacing the original data inputs as $z$ and training neural network $G^\prime(z)$ using the updated data $z$, then we can reduces the sample complexity from $\mathcal{S}(F, G, \mathcal{O}(\epsilon), \mathcal{O}(\delta)) \leq M$ to $\mathcal{S}(F, G^\prime, \mathcal{O}(\epsilon), \mathcal{O}(\delta)) \leq M(L-m)/L$.
\end{proposition}

Notice that the above analysis is under the assumption that the distribution of evaluation data is identical to the distribution of training data. However, this is often not the case in temporal data as the data distribution changes during time. 
To see whether data alignment could also improve the extrapolation ability, we provide a concrete example under the over-parameterized regime. 
Due to the space limit, we defer the discussion to Appendix~\ref{prop:data_alignment}.

In particular, we show that appropriate non-linearities of target function into the data could only improve the sample complexity of an 2-layer wide ReLU neural network of learning the polynomial function, but also help it extrapolate well when the input data distribution shifts.

\begin{corollary}\label{corollary:data_alignment_better_generalization}
Given a set of data points $\{\mathbf{x}_1,\ldots, \mathbf{x}_n\}$ with $\mathbf{x}_i\in\mathbb{R}^d$. Suppose the target function is a polynomial function defined as $F(\mathbf{x}) = \sum_{j=1}^m \alpha_j (\bm{\beta}_j^\top \mathbf{x})^p$ where $p\in\{2,4,6,8,\ldots\}$ is a positive even constant. Suppose we use a 2-layer ReLU neural network $G(\mathbf{x})  = \mathbf{v}_2^\top\sigma(\mathbf{W}_1 \mathbf{x}) $ to learn this target function $F(\mathbf{x})$, the sample complexity is  
\begin{equation}
    \mathcal{S}(F, G, \epsilon, \delta) = \mathcal{O}\left(\textcolor{red}{p} \times \frac{3}{\epsilon^2}\sum_{j=1}^m |\alpha_j| \| \bm{b}_j\|_2^p + \frac{\log(1/\delta)}{\epsilon^2}\right)
\end{equation}
It has been shown in~\cite{xu2020neural} that 2-layer ReLU neural network behaves like a linear function when the evaluation data is far from the training data. From Theorem~\ref{theorem:linear_extrapolation}, we know that 2-layer ReLU neural network $G$ cannot extrapolate the polynomial function $F$ if the evaluation data are from different distribution as the training data.

However, if we can encode the polynomial function into the data, i.e., the input data is $\mathbf{z}_i = \mathbf{x}_i^p$, use a 2-layer ReLU neural network $G^\prime(\mathbf{z})$ to learn this target function $F(\mathbf{x})$, then we can reduce the sample complexity to
\begin{equation}
    \mathcal{S}(F, G^\prime, \epsilon, \delta) = \mathcal{O}\left(\frac{3}{\epsilon^2}\sum_{j=1}^m  |\alpha_j| \| \bm{b}_j\|_2^p + \frac{\log(1/\delta)}{\epsilon^2}\right),
\end{equation}
which is smaller than $\mathcal{S}(F, G, \epsilon, \delta)$. 
 However, if we can encode the polynomial into data, i.e., replacing the original training data $\{ x_i \}_{i=1}^n$ as $\{ x_i^p \}_{i=1}^n$, then the objective function becomes linear with respect to the new training data $\{ x_i^p \}_{i=1}^n$, therefore it can extrapolate well.
 
\end{corollary}

\textcolor{blue}{======================\\}

\begin{theorem} [Linear extrapolation~\cite{xu2020neural}] \label{theorem:linear_extrapolation}
Let $G$ denote 2-layer ReLU neural network.
For any given direction $\mathbf{v}$, let define the input data $\mathbf{x}_1 = t\mathbf{v}, \mathbf{x}_2= \mathbf{x}_1 + h\mathbf{v} = (1+(h/t))\mathbf{v}$ for any $t,h > 0$. For $t\rightarrow \infty$, we have \smash{$\big| \frac{G(\mathbf{x}_1) - G(\mathbf{x}_2) }{h} - \epsilon \big| < \mathcal{O}\left(\frac{1}{t}\right)$},
where $\epsilon$ is a constant dependent on the direction $\mathbf{v}$.
\end{theorem}

\begin{assumption}\label{assumption:algorithmic_alignment_assmption}
We make the following assumption on neural network $G$ and training procedure:
\circled{1} Algorithm stability: Let denote $g, g^\prime$ as two neural network modules trained on two set of sampled data $\{(x_i, y_i)\}_{i=1}^M$ and $\{(x_i^\prime, y_i)\}_{i=1}^M$ respectively. Then, we suppose for any $\mathbf{z}$ there exists constant $C_0$ such that $\| g(x) - g^\prime(x) \|_2 \leq C_0 \cdot \max_{i\in[M]} \| x_i - x_i^\prime \|_2$
\circled{2} Sequential learning: Let suppose first train $g_1$ by $(x_i, f_1(x_i))$. Then, for any $\ell=2,\ldots, L$, we train the $\ell$-th neural network module $g_\ell$ by $(x_i^\prime, f_\ell(x_i^\prime))$ where $x_i^\prime = g_{\ell-1}(\ldots g_1(x_i)\ldots)$.
\circled{3} Lipschitzness: There exist constant $C_1$ such that $\|g_\ell(x) - g_\ell(x^\prime)\|_2 \leq L_1 \|x - x^\prime \|_2$ for any $\ell\in[L]$.

\end{assumption}
