# Supplementary material for: Do We Really Need Complicated Model Architectures For Temporal Networks?
Source: arXiv:2302.11636 source file (2023-02-22)
Supplement: Supplementary file 2 [file dynamic_of_link_prediction.tex]

Let $\mathcal{X}_i(k) = \{ (\mathbf{X}_i^\text{link}(k), \boldsymbol{t}_i(k)), \mathbf{x}_i^\text{spatial} \}$ denotes a set of inputs of our model. 
For simplicity, let drop the timestamp notation $k$.

Let $\mathcal{X}_i, \mathcal{X}_j$ denote a positive pair and $\mathcal{X}_i, \mathcal{X}_r$ denote a negative pair.

Let $\mathbf{z}_{i} = \text{Model}(\mathcal{X}_i, \boldsymbol{\theta})$ denotes the output of our model (parameterized by $\boldsymbol{\theta}$) on data $\mathcal{X}_i$. Therefore, $\mathbf{z}_i, \mathbf{z}_j$ is representation of a positive pair while $\mathbf{z}_i, \mathbf{z}_r$ is representation of a negative pair.

Let denote $p_{ij} = \langle \mathbf{z}_i, \mathbf{z}_j \rangle $.

During training, we are expecting the prediction of any positive pair $\mathbf{z}_i, \mathbf{z}_j$ is greater than the prediction of any negative pair $\mathbf{z}_i, \mathbf{z}_r$, i.e., 

\begin{equation}
    \begin{aligned}
    \mathcal{L}(\bm{\theta}) 
    &=  \sum_{(i,j)\in\mathcal{P}, (i,r) \in\mathcal{N}}  - \log\left(\frac{\exp(p_{ij})}{\exp(p_{ij}) + \exp(p_{ir})}\right) \\
    &= \sum_{(i,j)\in\mathcal{P}, (i,r) \in\mathcal{N}}  - \log\left(\frac{1}{1 + \exp(- p_{ij} + p_{ir})}\right) \\
    & = \sum_{(i,j)\in\mathcal{P}, (i,r) \in\mathcal{N}} - \log(\sigma(p_{ij}-p_{ir}))
    \end{aligned}
\end{equation}
where $\sigma(\cdot)$ is the sigmoid function.

During training, the gradient with respect to $\bm{\theta}$ can be computed as
\begin{equation}
    \begin{aligned}
    \frac{\partial \mathcal{L}(\bm{\theta})}{\partial \bm{\theta}} = \sum_{(i,j)\in\mathcal{P}, (i,r) \in\mathcal{N}} - \frac{\partial \log(\sigma(p_{ij}-p_{ir}))}{\partial \sigma(p_{ij}-p_{ir})}  \frac{\partial \sigma(p_{ij}-p_{ir})}{\partial p_{ij}}
    \end{aligned}
\end{equation}

We consider the classification problem as

\clearpage
\textcolor{red}{====================\\}

Inspired by~\cite{arora2019fine}.

Let consider the two layer neural network as
\begin{equation}
    \begin{aligned}
    f(\mathbf{x}_i) = \frac{1}{\sqrt{m}} \mathbf{a}^\top \text{ReLU}(\mathbf{W}^\top \mathbf{x}_i) 
    &= \frac{1}{\sqrt{m}} \sum_{r=1}^m a_r \text{ReLU}(\mathbf{w}_r^\top \mathbf{x}_i), \\
    &=\frac{1}{\sqrt{m}} \sum_{r=1}^m a_r \mathbb{I}\{\mathbf{w}_r^\top \mathbf{x}_i \geq 0\}(\mathbf{w}_r^\top \mathbf{x}_i)
    \end{aligned}
\end{equation}
where $\mathbf{W} = [\mathbf{w}_1,\ldots,\mathbf{w}_m] \in \mathbb{R}^{d\times m}$, $\mathbf{a} \in \mathbb{R}^m$, and $\mathbf{x}_i \in \mathbb{R}^d$.

Define the logistic regression as
\begin{equation}
    \begin{aligned}
    \ell(\mathbf{W}) &= \sum_{i=1}^n \log(1 + \exp( - y_i f(\mathbf{x}_i)) = \sum_{i=1}^n -\log(\sigma(y_i f(\mathbf{x}_i))) , \\
    \frac{\partial \ell(\mathbf{W})}{\partial \mathbf{w}_r} &= \frac{a_r}{\sqrt{m}}\sum_{i=1}^n \mu_i \mathbb{I}\{\mathbf{w}_r^\top \mathbf{x}_i \geq 0\} \mathbf{x}_i,~\mu_i = - y_i \sigma(-y_i f(\mathbf{x}_i))
    \end{aligned}
\end{equation}

The gradient descent is defined as
\begin{equation}
    \mathbf{w}_r(t+1) =  \mathbf{w}_r(t) - \eta \frac{\partial \ell(\mathbf{W}(t))}{\partial \mathbf{w}_r} \rightarrow \frac{\mathbf{w}_r(t+1) -  \mathbf{w}_r(t)}{\eta } = - \frac{\partial \ell(\mathbf{W}(t))}{\partial \mathbf{w}_r}
\end{equation}
By letting $\eta \rightarrow 0$ we have
\begin{equation}
    \frac{d\mathbf{w}_r(t)}{dt} = - \frac{\partial \ell(\mathbf{W}(t))}{\partial \mathbf{w}_r(t)}
\end{equation}

Let define symmetric matrix $\mathbf{H} \in \mathbb{R}^{n\times n}$ where the $i$-th row and $j$-th column is
\begin{equation}
    [\mathbf{H}]_{ij} = \frac{1}{m} \sum_{r=1}^m \mathbb{I}\{\mathbf{w}_r^\top \mathbf{x}_i \geq 0, \mathbf{w}_r^\top \mathbf{x}_j \geq 0\} \mathbf{x}_i^\top \mathbf{x}_j
\end{equation}

\textcolor{red}{
Define $\mathbf{H} = \mathbf{M}^\top \mathbf{M} \in \mathbb{R}^{n\times n}$, where $[\mathbf{H}]_{ij} = \frac{1}{m} \sum_{r=1}^m \mathbb{I}\{\mathbf{w}_r^\top \mathbf{x}_i \geq 0, \mathbf{w}_r^\top \mathbf{x}_j \geq 0\} \mathbf{x}_i^\top \mathbf{x}_j$ and
\begin{equation}
    \mathbf{M} = \begin{bmatrix}
\mathbb{I}\{\mathbf{w}_1^\top \mathbf{x}_1 \geq 0\} a_1 \mathbf{x}_1& \ldots & \mathbb{I}\{\mathbf{w}_1^\top \mathbf{x}_n \geq 0\} a_1 \mathbf{x}_n\\ 
\vdots & \ddots  & \vdots \\ 
\mathbb{I}\{\mathbf{w}_r^\top \mathbf{x}_1 \geq 0\} a_r \mathbf{x}_1 & \ldots & \mathbb{I}\{\mathbf{w}_r^\top \mathbf{x}_n \geq 0\} a_r \mathbf{x}_n 
\end{bmatrix} 
\in \mathbb{R}^{md\times n}
\end{equation}
}

Therefore, we have
\begin{equation}
    \begin{aligned}
    \frac{d f_t(\mathbf{x}_i)}{dt} &= \sum_{r=1}^m
    \left\langle  \frac{d f_t(\mathbf{x}_i)}{d\mathbf{w}_r(t)}, \frac{d\mathbf{w}_r(t)}{dt} \right\rangle \\
    &= \sum_{r=1}^m \left\langle \frac{1}{\sqrt{m}} a_r \mathbb{I}\{\mathbf{w}_r^\top(t) \mathbf{x}_i \geq 0\} \mathbf{x}_i, \frac{d \mathbf{w}_r(t)}{dt}\right\rangle \\
    &=  \sum_{r=1}^m \left\langle \frac{1}{\sqrt{m}} a_r \mathbb{I}\{\mathbf{w}_r^\top(t) \mathbf{x}_i \geq 0\} \mathbf{x}_i, - \frac{a_r}{\sqrt{m}}\sum_{j=1}^n \mu_j(t) \mathbb{I}\{\mathbf{w}_r^\top(t) \mathbf{x}_j \geq 0\} \mathbf{x}_j \right\rangle \\
    &=  - \frac{1}{m} \sum_{r=1}^m  \sum_{j=1}^n \mu_j(t) \mathbb{I}\{\mathbf{w}_r^\top(t) \mathbf{x}_i \geq 0, \mathbf{w}_r^\top(t) \mathbf{x}_j \geq 0\} \mathbf{x}_i^\top \mathbf{x}_j  \\
    &= - \sum_{j=1}^n [\mathbf{H}(t)]_{ij} \mu_j
    \end{aligned}
\end{equation}

Let $\mathbf{z} = [f(\mathbf{x}_1), \ldots, f(\mathbf{x}_n)] \in \mathbb{R}^n $. We have
\begin{equation}
    \frac{d \mathbf{z}(t)}{dt} = - \mathbf{H}(t) \bm{\mu} (t) 
    % = - \mathbf{H}(t) \cdot \mathbf{y} \cdot \sigma(- \mathbf{y} \cdot \mathbf{z}(t))
\end{equation}
and
\begin{equation}
    \frac{d \ell(\mathbf{W}(t))}{ dt} = \left\langle \frac{d \ell(\mathbf{W}(t))}{d \mathbf{z}(t)}, \frac{d \mathbf{z}(t)}{dt} \right\rangle  = - \bm{\mu}^\top (t) \mathbf{H}(t) \bm{\mu}(t) \leq - \lambda_{\min}(\mathbf{H}(t)) \| \bm{\mu}(t) \|_2^2
\end{equation}

\clearpage
