# Supplementary material for: Do We Really Need Complicated Model Architectures For Temporal Networks?
Source: arXiv:2302.11636 source file (2023-02-22)
Supplement: Supplementary file 3 [file generalization.tex]

\clearpage
\section{Generalization/extrapolation analysis} \label{section:generalization}

We first introduce the Rademacher complexity generalization bound by considering the difference between training and evaluation distribution, which is originally shown in The Corollary A.3 of~\cite{xu2021rethinking}. The corollary is adapted from the Theorem~1 of~\cite{koltchinskii2002empirical} and the Theorem 5 of~\cite{kakade2008complexity}. 

\begin{corollary} (Rademacher complexity with test distribution deviation) \label{corollary:train_eval_distribution_shift}
Consider an arbitrary function class $\mathcal{F}$ such that $\forall f\in\mathcal{F}$ we have $\sum_{x \in \mathcal{X}} |f(x)| \leq C$. Then, with probability at least $1-\delta$ over the sample, for all margins $\gamma > 0$ and all $f\in\mathcal{F}$ we have,
\begin{equation*}
    P_\text{eval}(y f(x) \leq 0) \leq \frac{1}{n} \sum_{i=1}^n \eta(x_i) \mathbf{1}\{y_i f(x_i) < \gamma \}  + \frac{4 \mathfrak{R}_\eta(\mathcal{F})}{\gamma} + Q(\epsilon, \delta, C),
\end{equation*}
where $\eta(x), \mathfrak{R}_{n,\eta}(\mathcal{F}), Q(\epsilon, \delta, C)$ are defined as
\begin{equation*}
    \eta(x) = \frac{P_\text{eval}(x)}{P_\text{train}(x)},~
    \mathfrak{R}_\eta(\mathcal{F}) = \mathbb{E}\left[\sup_{f\in\mathcal{F}} \eta(x_i) f(x_i) \epsilon_i\right],~
    Q(\epsilon, \delta, C) = \sqrt{\frac{\log(\log(4C/\gamma))}{n}} + \sqrt{\frac{\log(1/\delta)}{2n}}.
\end{equation*}
\end{corollary}

From Corollary~\ref{corollary:train_eval_distribution_shift}, we know that 
\begin{equation*}
    \mathcal{R}_\text{eval}(f) \leq \mathcal{R}_\text{train}^\gamma(f) + D_{\ell_1} + \frac{4\mathfrak{R}_\eta(\mathcal{F})}{\gamma} + Q(\epsilon,\delta,C)
\end{equation*}
Then, the remaining left is to upper bound the model complexity term $\mathfrak{R}_\eta(\mathcal{F})$, which follows the proof of Theorem 4 of~\cite{koltchinskii2002empirical}.

\weilin{might need to write details on it}
