# Supplementary material for: Do We Really Need Complicated Model Architectures For Temporal Networks?
Source: arXiv:2302.11636 source file (2023-02-22)
Supplement: Supplementary file 4 [file uniform_approximation.tex]

\begin{theorem} [Uniform approximation] \label{theorem:mlp_mixer_uniform_approx}
Let $p\in[1, +\infty)$ and $\epsilon >0$, then for any $f\in\mathcal{F}$, there exists a MLP-mixer $g$ such that $\text{dist}(f,g) \leq \epsilon$, where $\text{dist}(f,g) := (\int \| f(\mathbf{X}) - g(\mathbf{X}) \|_p^p d\mathbf{X})^{1/p}$.
\end{theorem}

To begin with, we theoretically show in Theorem~\ref{theorem:mlp_mixer_uniform_approx} that the MLP-mixer can uniform approximate any \textit{continuous function} defined on $\mathbf{T}_i(t_0)$, where $\mathbf{T}_i(t_0)$ is the temporal link information of any node $v_i$ as introduced in Section~\ref{section:temporal_encoder}.
To the best of our knowledge, this is the first analysis of the uniform approximation ability of MLP-mixer for sequence data.

\weilin{add a proof sketch + some intuitions}
\weilin{this part seems non-trivial if following previous work's idea ...}

Although Theorem~\ref{theorem:mlp_mixer_uniform_approx} indicates the strong expressiveness of using MLP-mixer,

\section{MLP-mixer uniform approximate any continuous function defined on sequence}

\subsection{Approximate any continuous function $\mathcal{F}$ with piece-wise constant function}

Let us define $\delta > 0$, grid $\mathbb{G}_\delta := \{0, \delta, 2\delta,\ldots, 1-\delta\}^{d\times n}$ and the associated cube of wide $\delta$ as $\mathbb{S}_\mathbf{L} = \prod_{i=1}^d \prod_{j=1}^n [[\mathbf{L}]_{ij}, [\mathbf{L}]_{ij}+ \delta) \subset [0, 1]^{d\times n}$.
Then, given any $\mathbf{L} \in \mathbb{G}_\delta$, we defined the indicator function as $\mathbb{I}\{\mathbf{X} \in \mathbb{S}_\mathbf{L}\}$ where it returns $1$ if $[\mathbf{X}]_{ij} \in [[\mathbf{L}]_{ij}, [\mathbf{L}]_{ij}+\delta),~\forall i\in[d], j\in[n]$ and it returns $0$ otherwise. 
In the following, we first show in Lemma~\ref{section:uniform_approx_step_1} that any continuous function $\mathcal{F}$ can be approximate arbitrary accurate by piece-wise constant function $\bar{\mathcal{F}}(\delta)$, where
\begin{equation*}
    \bar{\mathcal{F}}(\delta) := \left\{ f: \mathbf{X} \rightarrow \sum_{\mathbf{L \in \mathbb{G}_\delta}} \mathbf{A}_\mathbf{L} \times \mathbb{I}\{\mathbf{X} \in \mathbb{S}_\mathbf{L}\}~|~\mathbf{A}_\mathbf{L} \in \mathbb{R}^{d\times n}\right\}.
\end{equation*}

\begin{lemma} [Lemma 8 of~\cite{Yun2020Are}] \label{section:uniform_approx_step_1}
For any continous function $f\in\mathcal{F}$ and $1\leq p < \infty$, we can always find a $\delta^\star$ such that $\exists \bar{f} \in \bar{\mathcal{F}}(\delta^\star)$ which satisfies $\text{dist}(f, \bar{f}) \leq \epsilon /3 $.
\end{lemma}

\subsection{Approximate $\bar{\mathcal{F}}(\delta)$ with modified MLP-mixer}

\subsubsection{Quantization by channel mixer layers}

Instead of using ReLU in the original MLP-mixer model, we consider two types of element-wise activations:
\begin{equation*}
    \sigma_1(t) = \begin{cases}
-t - \delta ^{-nd} & \text{ if } t < 0~\text{or}~t \geq 1 \\ 
0 & \text{ otherwise } 
\end{cases},~
\sigma_2(t) = \begin{cases}
-t+k\delta  & \text{ if } 0 \leq t-k\delta < \delta \\ 
0 & \text{ otherwise } 
\end{cases}
\end{equation*}

In this section, we will show that given a piece-wise constant function $\bar{f} \in \bar{\mathcal{F}}(\delta)$. there exists a modified MLP-mixer $\bar{g}$ that closely approximate $\bar{f}$.

Given an input $\mathbf{X} \in \mathbb{R}^{d\times n}$, a series of channel mixer layers can quantize $\mathbf{X}$ to an element $\mathbf{L}$ on the extended grid $\mathbb{G}_\delta^+ := \{-\delta^{-nd}, 0, \delta, 2\delta,\ldots, 1-\delta\}^{d\times n}$

% \begin{lemma} [Lemma 5 of~\cite{Yun2020Are}] \label{section:uniform_approx_step_2_1}
% Consider a scalar quantization map $g_q^\text{ent}: \mathbb{R} \rightarrow \{-\delta^{-nd}, 0, \delta, 2\delta,\ldots, 1-\delta\}$ that
% \begin{equation*}
%     g_q^\text{ent}:= \begin{cases}
%     k\delta & \text{ if } k\delta \leq t \leq (k+1)\delta,~ k\in\{0, \delta, 1/\delta - 1\} \\ 
%     -\delta^{-nd} & \text{ otherwise } 
%     \end{cases}
% \end{equation*}
% There exists a function $g_q: \mathbb{R}^{n\times d} \rightarrow \mathbb{G}_\delta^+$ composed of $(1+\frac{1}{\delta})$ channel mixer layers with hidden dimension as $d$ (the first layers uses $\sigma_1$ and others use $\sigma_2$ as activation), which employs the scalar quantization $g_q^\text{ent}$ to each entry of its input, where $g_q$ maps any $\mathbf{X}\in\mathbb{S}_\mathbf{L}$ to $\mathbf{L}$ and set the other elements in $\mathbf{X}$ that are not in $[0,1]$ to $-\delta^{-nd}$.
% \end{lemma}

\begin{lemma} [Lemma 5 of~\cite{Yun2020Are}] \label{section:uniform_approx_step_2_1}
There exists a function $g_q: \mathbb{R}^{d\times n} \rightarrow \mathbb{G}_\delta^+$ that is composed of $(1+\frac{1}{\delta})$ channel mixer layers with hidden dimension as $d$ (the first layers uses $\sigma_1$ and others use $\sigma_2$ as activation) could maps any $\mathbf{X}\in\mathbb{S}_\mathbf{L}$ to $\mathbb{G}_\delta^+$ by applying $g_q^\text{element}(t)$ onto each element of $\mathbf{X}$:
\begin{equation*}
    g_q^\text{element}(t):= \begin{cases}
    k\delta & \text{ if } k\delta \leq t \leq (k+1)\delta,~ k\in\{0, \delta, 1/\delta - 1\} \\ 
    -\delta^{-nd} & \text{ otherwise } 
    \end{cases}
\end{equation*}
\end{lemma}

\subsubsection{Contextual mapping by token-mixer layers}

In this section, we show that the token-mixer layer in the modified MLP-mixer can compute contextual mappings from the output of $g_q$ by using composition of token-mixer layers, where the contextual mapping is defined as following:

\begin{definition} [Contextual mapping] A mapping $q: \mathbb{G}_\delta^+ \rightarrow \mathbb{R}^{1\times n}$ is contextual mapping if (1) For any $\mathbf{L} \in \mathbb{G}_\delta^+$, the $n$ entries in $q(\mathbf{L})$ are all distinct; (2) For any $\mathbf{L},\mathbf{L}^\prime \in \mathbb{G}_\delta^+$ with $\mathbf{L} \neq \mathbf{L}^\prime$, all entries of $q(\mathbf{L})$ and $q(\mathbf{L}^\prime)$ are distinct.
\end{definition}

The key to the proof is to show inter-changing use of token mixer and channel mixer can achieve contextual mapping.
